# Supplementary material for: Modelling intransitivity in pairwise comparisons with application to baseball data
Source: arXiv:2103.12094 source file (2023-02-16)
Supplement: Supplementary file 1 [file RJ_supplimentary.pdf]

# Supplementary material for “Modelling intransitivity in pairwise comparisons with application to baseball data”: reversible jump Markov chain Monte Carlo algorithm

Harry Spearing, Jonathan Tawn

Lancaster University

March 22, 2021

## S:1 Overview

This document contains the full details of the reversible jump Markov chain Monte Carlo (RJMCMC) algorithm (Green, 1995) used for inference in the article “Modelling intransitivity in pairwise comparisons with application to baseball data”.

The RJMCMC sampler provides samples from the posterior distribution  $\pi(\boldsymbol{\phi}, \mathbf{Y}, A, \boldsymbol{\theta}, \mathbf{Z}, K | \mathbf{x})$ , that is, the intransitivity and skill levels, the allocations to the these levels, and the number of levels. Specifically, a split-merge sampler (Green and Richardson, 2001) is used, which is adapted from the work of Ludkin (2020). The sampler comprises three separate moves: a standard MCMC Metropolis-Hastings move, which samples parameters  $\boldsymbol{\phi}, \boldsymbol{\theta}$ , and reallocates clusters  $\mathbf{Y}, \mathbf{Z}$ ; splitting or merging clusters; and adding or deleting empty clusters. Let  $(\boldsymbol{\phi}^s, \mathbf{Y}^s, A^s, \boldsymbol{\theta}^s, \mathbf{Z}^s, K^s)$  be the current values of the parameters at step  $s$  in the sampler, and for any move a proposal  $(\boldsymbol{\phi}', \mathbf{Y}', A', \boldsymbol{\theta}', \mathbf{Z}', K')$  is made. To be concrete,

$$\begin{aligned}\boldsymbol{\phi}^s &= \{\phi_a^s : a \in \{-A_-^s, \dots, A_+^s\}\} \\ \mathbf{Y}^s &= \{\mathbf{y}_{\{i\}}^s : i \in \mathcal{I} \setminus \{1\}\} \\ \boldsymbol{\theta}^s &= \{\theta_k^s : k \in \{1, \dots, K^s\}\} \\ \mathbf{Z}^s &= \{\mathbf{z}_{\{i,j\}}^s : i > j \in \mathcal{I} \setminus \{1\}\},\end{aligned}$$

where  $\mathbf{z}_{\{i,j\}}^s = \{z_{\{i,j\},a}^s : a \in \{-K^s, \dots, K^s\}\}$ , for all steps  $s \in \{1, \dots, S\}$  in the sampler where  $S \in \mathbb{N}$ .

As discussed in Section 4.2, the clustering of our two features - the skills of the objects and the intransitivity of the pairs of objects - are treated as independent systems. Therefore we approach them separately: all of Sections S:2.1, S:3.1 and S:4.1 outline the intransitivity components of the algorithm, and Section S:2.2, S:3.2 and S:4.2 outline their skill component counterparts.

## S:2 Split-Merge components

### S:2.1 Split-Merge components : intransitivity

#### S:2.1.1 Intransitivity split move

To split an intransitivity cluster, first a cluster must be chosen to split, and this is chosen at random. A potentially more efficient proposal could be made by proposing to split a cluster,

say, proportional to cluster size or as a function of its vicinity to neighbouring clusters. For simplicity, in this article all clusters in split and merge moves are randomly selected with equal probability.

Let the cluster to be split be denoted as  $k \in \{0, \dots, K\}$ , with intransitivity level  $\theta_k^s \in \boldsymbol{\theta}_K$  and the proposed new clusters be  $k'$  and  $k' + 1$  with intransitivity levels  $\theta_{k'}^s, \theta_{k'+1}^s \geq 0$ , respectively, so that the proposed intransitivity levels are  $\boldsymbol{\theta}' = \{\theta_0^s, \dots, \theta_{k-1}^s, \theta_{k'}^s, \theta_{k'+1}^s, \theta_{k+1}^s, \dots, \theta_K^s\}$ . This notation is chosen because the ordering of the clusters must be maintained, for example  $\theta_{k-1}^s < \theta_{k'}^s < \theta_{k'+1}^s < \theta_{k+1}^s$ , to avoid label switching issues in the inference. Note that with this notation, the transitive cluster can be split, however in this case, one of the proposed intransitivity levels must be 0, to maintain the generalisation to a Bradley-Terry model. The proposed number of clusters is of course  $K' = K^s + 1$ .

Next, the new cluster parameters are proposed. To preserve ordering, consider the transformation of  $\theta_k^s$ ,  $k \neq 0$  such that the allowed range of  $\theta_k^s$  changes from  $(\theta_{k-1}^s, \theta_{k+1}^s)$  to  $(-\infty, \infty)$ . Then, a new intransitivity level is proposed on this scale, and then transformed back to the its original range  $(\theta_{k-1}^s, \theta_{k+1}^s)$ . If  $k = K^s$ , then the range  $(\theta_{K^s-1}^s, \theta_{K^s+1}^s)$  is currently undefined because  $\theta_{K^s+1}^s$  is undefined. Therefore we introduce a

$$\theta_{K^s+1}^s := \theta_{K^s}^s + (\theta_{K^s}^s - \theta_{K^s-1}^s) = 2\theta_{K^s}^s - \theta_{K^s-1}^s, \quad (\text{S.1})$$

which acts as an upper bound for the proposed new intransitivity levels  $\theta_{k'}^s, \theta_{k'+1}^s$  such that  $\max(\theta_{k'+1}^s) = 2\theta_{K^s}^s - \theta_{K^s-1}^s$ . Thus  $\theta_{k'+1}^s$  cannot increase by more than  $\theta_{K^s}^s - \theta_{K^s-1}^s$ , which is also the maximum  $\theta_{k'}^s$  can decrease by without violating the ordering constraint. If  $k = 0$ , i.e., the completely transitive cluster has a split proposed, then the lower proposed level must be  $\theta_{0'}^s = 0$ , but the level  $\theta_{1'}^s$  follows the same rules as for a general  $k \neq 0$ , described below, therefore upper and lower bounds are defined for all values in  $\boldsymbol{\theta}^s$ .

The transformation onto the range  $(-\infty, \infty)$  is achieved using a *matching function*  $y(\theta_k^s | \theta_{k-1}^s, \theta_{k+1}^s)$ , defined as

$$y(x | \theta_{k-1}^s, \theta_{k+1}^s) = \text{logit} \left( \frac{x - \theta_{k-1}^s}{\theta_{k+1}^s - \theta_{k-1}^s} \right), \quad k \in \{1, \dots, K\}, \quad x \in (\theta_{k-1}^s, \theta_{k+1}^s), \quad (\text{S.2})$$

where  $\text{logit}(a) = \log(a/(1-a))$ ,  $a \in [0, 1]$ . Then, the *auxiliary variable*  $u \sim \sigma \chi_1^2$ , for  $\sigma > 0$ , is added (and subtracted) to the transformed intransitivity level to give the proposed upper (and lower) transformed intransitivity levels, respectively, such that

$$y(\theta_{k'+1}^s | \theta_{k-1}^s, \theta_{k+1}^s) = y(\theta_k^s | \theta_{k-1}^s, \theta_{k+1}^s) + u \quad (\text{S.3})$$

$$y(\theta_{k'}^s | \theta_{k-1}^s, \theta_{k+1}^s) = y(\theta_k^s | \theta_{k-1}^s, \theta_{k+1}^s) - u. \quad (\text{S.4})$$

After a retransformation back to the original scale, this gives values of the lower and upper proposed intransitivity levels  $\theta_{k'}^s$  and  $\theta_{k'+1}^s$ , with  $\theta_{k-1}^s < \theta_{k'}^s < \theta_{k'+1}^s < \theta_{k+1}^s$ , as

$$\theta_{k'}^s = \begin{cases} \frac{\theta_{k-1}^s + \theta_{k+1}^s \exp(-u) (\theta_k^s - \theta_{k-1}^s) / (\theta_{k+1}^s - \theta_k^s)}{1 + \exp(-u) (\theta_k^s - \theta_{k-1}^s) / (\theta_{k+1}^s - \theta_k^s)} & \text{if } k' \neq 0' \\ 0 & \text{if } k' = 0' \end{cases} \quad (\text{S.5})$$

$$\theta_{k'+1}^s = \frac{\theta_{k-1}^s + \theta_{k+1}^s \exp(u) (\theta_k^s - \theta_{k-1}^s) / (\theta_{k+1}^s - \theta_k^s)}{1 + \exp(u) (\theta_k^s - \theta_{k-1}^s) / (\theta_{k+1}^s - \theta_k^s)}. \quad (\text{S.6})$$

Equations (S.5) and (S.6) are the main contributions to ensure that ordering and labelling is preserved in RJMCMC type algorithms.

The next state of the sampler  $(\boldsymbol{\phi}^{s+1}, \mathbf{Y}^{s+1}, A^{s+1}, \boldsymbol{\theta}^{s+1}, \mathbf{Z}^{s+1}, K^{s+1})$  is then accepted to be  $(\boldsymbol{\phi}^s, \mathbf{Y}^s, A^s, \boldsymbol{\theta}', \mathbf{Z}', K')$  with some probability  $A_{split}$ , and otherwise

$$(\boldsymbol{\phi}^{s+1}, \mathbf{Y}^{s+1}, A^{s+1}, \boldsymbol{\theta}^{s+1}, \boldsymbol{\theta}^{s+1}, \mathbf{Z}^{s+1}, K^{s+1}) = (\boldsymbol{\phi}^s, \mathbf{Y}^s, A^s, \boldsymbol{\theta}^s, \mathbf{Z}^s, K^s).$$

The form of the acceptance probability  $A_{split}$  is computed as:

$$\begin{aligned} A_{split} &= \frac{\pi(\boldsymbol{\phi}^s, \mathbf{Y}^s, A^s, \boldsymbol{\theta}', \mathbf{Z}', K^s + 1 | \mathbf{x})}{\pi(\boldsymbol{\phi}^s, \mathbf{Y}^s, A^s, \boldsymbol{\theta}^s, \mathbf{Z}^s, K^s | \mathbf{x})} \frac{q(K^s, \mathbf{Z}^s, \boldsymbol{\theta}^s | K^s + 1, \mathbf{Z}', \boldsymbol{\theta}')}{q(K^s + 1, \mathbf{Z}', \boldsymbol{\theta}' | K^s, \mathbf{Z}^s, \boldsymbol{\theta}^s)} \frac{1}{q_u(u)} J_{split} \\ &= \frac{\pi(\boldsymbol{\phi}^s, \mathbf{Y}^s, A^s, \boldsymbol{\theta}', \mathbf{Z}', K^s + 1 | \mathbf{x})}{\pi(\boldsymbol{\phi}^s, \mathbf{Y}^s, A^s, \boldsymbol{\theta}^s, \mathbf{Z}^s, K^s | \mathbf{x})} \frac{q(merge | K^s + 1)}{q(split | K^s)} \frac{q_k(k', k' + 1)}{q_k(k)} \frac{1}{q_u(u)} \frac{1}{q(\mathbf{Z}')} J_{split}, \quad (\text{S.7}) \end{aligned}$$

which is the ratio of the posterior densities, the ratio of the proposal densities, and the ratio of the densities of the auxiliary variables and the Jacobian,  $J_{split}$ . If  $K^s = 0$ , then the probability of proposing a *merge*, see Section S:2.1.2, is  $q(merge | K^s = 0) = 0$  and the probability of proposing a split  $q(split | K^s = 0) = 1$ . Otherwise,  $q(merge | K^s \neq 0) = q(split | K^s \neq 0) = 1/2$ , and therefore the ratio of is simply

$$\frac{q(merge | K^s + 1)}{q(split | K^s)} = \frac{1}{1 + \mathbb{1}\{K^s = 0\}}.$$

The probability of selecting cluster  $k$  to split is  $q_k(k) = \frac{1}{K^s}$ ,  $\forall k \in \{1, \dots, K^s\}$ . The probability of selecting clusters  $k', k' + 1$ ,  $\forall k' \in \{1, \dots, K' - 1\}$  to be merged back again is also  $q_k(k', k' + 1) = \frac{1}{K' - 1} = \frac{1}{K^s}$ , so these terms will cancel. The density of the auxiliary variables is the density of  $u$ ,  $q_u(u)^{-1}$ , which is given as  $\chi_1^2(u/\sigma)$ , where  $\chi_1^2(x)$  is the density of a chi-squared distribution with 1 degree of freedom.

The probability of the allocations is  $q(\mathbf{Z}')$ , and this is dependent on the cluster being split and the current state of the model, for which there are three different situations to consider:

#### The general case: ( $k \neq 0$ )

Since the transitive level  $\theta_0 = 0$  adds additional complications, we first depict the acceptance probability for the general case that  $k \neq 0$ . Let  $\mathbf{b}_k^s = \{\{i, j\}, \forall i > j \in \mathcal{I} \setminus \{1\} : z_{\{i, j\}, k}^s = 1\}$  denote the set of pairs  $i > j \in \mathcal{I} \setminus \{1\}$  of objects which belong to the cluster-to-be-split, i.e.,  $k \neq 0$ . Then, the probability of the cluster allocation, given that cluster  $k \neq 0$  has been split,

$$q(\mathbf{Z}') = \left( \frac{|\mathbf{b}_k^s|!}{|\mathbf{b}'_{k'}|! |\mathbf{b}'_{k'+1}|!} \right) 2^{-(|\mathbf{b}_k^s|)} \left( \frac{|\mathbf{b}_{-k}^s|!}{|\mathbf{b}'_{-k'}|! |\mathbf{b}'_{-(k'+1)}|!} \right) 2^{-(|\mathbf{b}_{-k}^s|)}$$

since the new cluster allocations are selected at random and all possible combinations of allocation must be considered, and remembering that cluster  $-k$  will also be split into clusters  $-k'$  and  $-k' - 1$  with intransitivity levels  $\theta'_{-k'} = -\theta'_{k'}$  and  $\theta'_{-k'-1} = -\theta'_{k'+1}$ . See Appendix S:A.1 for details of the Jacobian  $J_{split}$ . Combining these components, the acceptance probability of splitting a cluster  $k \neq 0$  can be computed as

$$A_{split} | (k \neq 0) = \Lambda_{split} \left( \frac{|\mathbf{b}_k^s|! |\mathbf{b}_{-k}^s|! 2^{-(|\mathbf{b}_k^s| + |\mathbf{b}_{-k}^s|)}}{|\mathbf{b}'_{k'}|! |\mathbf{b}'_{k'+1}|! |\mathbf{b}'_{-k'}|! |\mathbf{b}'_{-(k'+1)}|!} \right)^{-1} J_{split}, \quad (\text{S.8})$$

where

$$\Lambda_{split} = \frac{\pi(\boldsymbol{\phi}^s, \mathbf{Y}^s, A^s, \boldsymbol{\theta}', \mathbf{Z}', K^s + 1 | \mathbf{x})}{\pi(\boldsymbol{\phi}^s, \mathbf{Y}^s, A^s, \boldsymbol{\theta}^s, \mathbf{Z}^s, K^s | \mathbf{x})} \frac{1}{1 + \mathbb{1}\{K^s = 0\}} \frac{\sigma}{\chi_1(u/\sigma)}.$$

#### Splitting from the transitive cluster: ( $k = 0$ , $K^s \geq 1$ )

We now consider the special case that we propose to split the transitive cluster ( $k = 0$ ), when there are other intransitive clusters ( $K^s \geq 1$ ). The acceptance probability for this proposal differs slightly, because  $\theta_0 = 0$  is fixed. If a split is proposed on level 0 with intransitivity level  $\theta_0^s$ , then the proposed clusters are  $0'$  and  $1'$  with intransitivity levels  $\theta'_{0'}, \theta'_{1'}$ ; however, the completely transitive level must remain so, in order that the model remains an exact generalisation of the Bradley-Terry model, that is  $\theta'_{0'} = \theta_0 = 0$ . The level  $1'$  has intransitivity level  $\theta'_{1'} > 0$  governed by equation (S.6), remembering that  $\theta'_{-1} = -\theta'_{1'}$ . Additionally, a separate Jacobian  $J_{split,0}$  is

required, see Appendix S:A.3. The cluster allocation also differs. Instead of allocating pairs in  $k$  to either  $k', k' + 1$  and pairs in  $-k$  to either  $-k', -k' + 1$ , the pairs in 0 are allocated to one of  $0', -1', 1'$ . The probability of the cluster allocation is therefore

$$q_0(\mathbf{Z}') = \left( \frac{|\mathbf{b}_0^s|!}{|\mathbf{b}_{-1}^s|! |\mathbf{b}_0^s|! |\mathbf{b}_1^s|!} \right) 3^{-|\mathbf{b}_0^s|},$$

since the allocation is at random. This gives an acceptance probability of

$$A_{split}|(k = 0, K^s \geq 1) = \Lambda_{split} \left( \frac{|\mathbf{b}_0^s|!}{|\mathbf{b}_{-1}^s|! |\mathbf{b}_0^s|! |\mathbf{b}_1^s|!} \right)^{-1} \left( \frac{1}{3} \right)^{-|\mathbf{b}_0^s|} J_{split,0}, \quad (\text{S.9})$$

if  $k = 0, K^s \geq 1$ .

### Splitting from the Bradley-Terry case: ( $K^s = 0$ )

Consider the special case that only the transitive level exists and therefore the model in this state is identical to the Bradley-Terry. The transformation via the matching function, equation (S.2), is not possible in this case since the bounds  $\theta_{K^s+1}^s$  (and  $\theta_{-(K^s+1)}^s = -\theta_{K^s+1}^s$ ) are not defined when  $K^s = 0$ . However, ordering is not an issue in this case, and so the levels are simply proposed as

$$\theta'_{0'} = \theta_0, \quad \theta'_{1'} = \theta_0 + u = u,$$

which gives a Jacobian of 1, and where  $u$  is still defined as  $u \sim \sigma \chi_1^2$ , and the pairs in 0 are again allocated to one of  $0', 1', -1'$ . Therefore the acceptance probability, for  $K^s = 0$ , is given as

$$A_{split}|(K^s = 0) = \Lambda_{split} \left( \frac{|\mathbf{b}_0^s|!}{|\mathbf{b}_{-1}^s|! |\mathbf{b}_0^s|! |\mathbf{b}_1^s|!} \right)^{-1} \left( \frac{1}{3} \right)^{-|\mathbf{b}_0^s|}. \quad (\text{S.10})$$

### S:2.1.2 Intransitivity merge move

So as to not confuse notation, we will consider the merge in terms of a reversed split move. Therefore let  $(\boldsymbol{\phi}^s, \mathbf{Y}^s, A^s, \boldsymbol{\theta}', \mathbf{Z}', K') = (\boldsymbol{\phi}^{s+1}, \mathbf{Y}^{s+1}, A^{s+1}, \boldsymbol{\theta}^{s+1}, \mathbf{Z}^{s+1}, K^{s+1})$  be the current values of the parameters at step  $s$ , and we aim to propose parameters  $(\boldsymbol{\phi}^s, \mathbf{Y}^s, A^s, \boldsymbol{\theta}^s, \mathbf{Z}^s, K^s)$ . Two clusters are sampled to merge, however, since these must be consecutive clusters, in order to preserve order, we can simply sample from the set  $k' \sim \{0, \dots, K' - 1\}$  and then merge clusters  $k'$  and  $k' + 1$  into a new cluster  $k$ . Again there are many other ways to propose which clusters to merge, but for now we sample with equal probability. The proposed number of clusters must be  $K^s = K' - 1$ . Next, the cluster membership  $\mathbf{Z}^s$  is updated which is simple because all pairs of objects from both clusters  $k'$  or  $k' + 1$  get assigned to the new cluster  $k$ . To find a suitable cluster mean  $\theta_k^s$ , the inverse of the split move is used, so inversely to the split move, the matching function

$$y(x|\theta'_{k'-1}, \theta'_{k'+2}) = \text{logit} \left( \frac{x - \theta'_{k'-1}}{\theta'_{k'+2} - \theta'_{k'-1}} \right), \quad x \in (\theta'_{k'-1}, \theta'_{k'+2}), \quad (\text{S.11})$$

is used. Then the proposed merged transformed cluster mean is given from equations (S.3) and (S.4), as

$$y(\theta_k^s|\theta'_{k'-1}, \theta'_{k'+2}) = \frac{[y(\theta'_{k'}|\theta'_{k'-1}, \theta'_{k'+2}) + y(\theta'_{k'+1}|\theta'_{k'-1}, \theta'_{k'+2})]}{2}, \quad (\text{S.12})$$

which results in a proposed merged cluster mean of

$$\theta_k^s = \theta'_{k'-1} + \frac{(\theta'_{k'+2} - \theta'_{k'-1})}{1 + \left[ \left( \frac{\theta'_{k'} - \theta'_{k'-1}}{\theta'_{k'+2} - \theta'_{k'}} \right) \left( \frac{\theta'_{k'+1} - \theta'_{k'-1}}{\theta'_{k'+2} - \theta'_{k'+1}} \right) \right]^{-1/2}}. \quad (\text{S.13})$$

Then, the next state is accepted to be  $(\boldsymbol{\phi}^s, \mathbf{Y}^s, A^s, \boldsymbol{\theta}^s, \mathbf{Z}^s, K^s) = (\boldsymbol{\phi}^s, \mathbf{Y}^s, A^s, \boldsymbol{\theta}', \mathbf{Z}', K')$ , with probability  $A_{merge}$ , whose precise form depends the situation.

### The general case: ( $k' \neq 0$ )

In the most general case, that  $k' \neq 0$ , then this gives an acceptance probability of

$$A_{merge}|(k' \neq 0) = \Lambda_{merge} \left( \frac{\mathbf{b}_k^s! \mathbf{b}_{-k}^s! 2^{-(|\mathbf{b}_k^s| + |\mathbf{b}_{-k}^s|)}}{\mathbf{b}_{k'}^s! \mathbf{b}_{k'+1}^s! \mathbf{b}_{-k'}^s! \mathbf{b}_{-(k'+1)}^s!} \right) (J'_{split})^{-1}, \quad (\text{S.14})$$

where

$$\Lambda_{merge} = \frac{\pi(\boldsymbol{\phi}^s, \mathbf{Y}^s, A^s, \boldsymbol{\theta}^s, \mathbf{Z}^s, K' - 1 | \mathbf{x})}{\pi(\boldsymbol{\phi}^s, \mathbf{Y}^s, A^s, \boldsymbol{\theta}', \mathbf{Z}', K' | \mathbf{x})} (1 + \mathbb{1}\{K' = 1\}) \frac{\chi_1(u'/\sigma)}{\sigma},$$

and where  $u' = y(\theta'_{k'+1} | \theta'_{k'-1}, \theta'_{k'+2}) - y(\theta_k^s | \theta'_{k'-1}, \theta'_{k'+2})$  is the value required for the inverse split move to get back to intransitivity levels  $\theta'_{k'}$  and  $\theta'_{k'+1}$ , and  $J'_{split}$  is the Jacobian for the inverse split move. This gives the acceptance probability for a merge when  $k' \neq 0$ , however, like the split move, there are two other variants, outlined below.

### Merging to the transitive cluster: ( $k' = 0, K' \geq 2$ )

If  $k' = 0$ , and therefore clusters  $0', 1'$  are being merged to cluster 0 with intransitivity level  $\theta_k^s = \theta_0^s = 0$ , then, similarly to the equivalent split move, the allocation probability changes because pairs from  $0', -1', 1'$  are proposed to move into 0. The Jacobian also changes to  $J'_{split,0}$ , see Appendix S:A.3, and the acceptance probability is given as

$$A_{merge}|(k' = 0, K' \geq 2) = \Lambda_{merge} \left( \frac{|\mathbf{b}_0^s|!}{|\mathbf{b}_{-1}^s|! |\mathbf{b}_0^s|! |\mathbf{b}_1^s|!} \right) \left( \frac{1}{3} \right)^{|\mathbf{b}_0^s|} (J'_{split,0})^{-1}. \quad (\text{S.15})$$

### Merging to the Bradley-Terry case: ( $K' = 1$ )

Similarly to the equivalent split move, if  $K' = 1$ , then the proposed merge move would be to a Bradley-Terry model (or generalisation thereof). In this case no transformation is required, and thus no Jacobian term, and so

$$A_{merge}|(K' = 1) = \Lambda_{merge} \left( \frac{|\mathbf{b}_0^s|!}{|\mathbf{b}_{-1}^s|! |\mathbf{b}_0^s|! |\mathbf{b}_1^s|!} \right) \left( \frac{1}{3} \right)^{|\mathbf{b}_0^s|}, \quad (\text{S.16})$$

where in this case  $u' = \theta'_{k'+1}$ .

## S:2.2 Split-Merge components : skill

### S:2.2.1 Skill split move

The split and merge components are now considered for the objects skill levels. The reversible jump moves here are similar to those of the intransitivity levels, but a few changes are needed to accommodate for the fact that levels can have either positive or negative values, and that symmetry in the skill levels is not enforced as it is for the intransitivity levels. A cluster  $a \in \mathcal{A}^s$  is selected at random to be split, with a skill level  $\phi_a^s \in \boldsymbol{\phi}^s$ , and the proposed new clusters are labelled  $a', a' + 1$ , and have skill levels  $\phi'_{a'}, \phi'_{a'+1} \in \mathbb{R}$ . Note that the skill level  $\phi_0 = 0$  can be split, although in this case one of the proposed skill levels must also be 0, and object 1 must stay in this level. The proposed number of skill levels is of course  $A' = A^s + 1$ . Next, the new skill level parameters are proposed.

From the current allocations  $\mathbf{Y}^s$ , the proposed allocations  $\mathbf{Y}'$  are found by randomly reallocating those objects in cluster  $a$  to either cluster  $a'$  or  $a' + 1$  with equal probability.

The acceptance probability  $A_{split_A}$  is then computed as:

$$\begin{aligned} A_{split_A} &= \frac{\pi(\boldsymbol{\phi}', \mathbf{Y}', A^s + 1, \boldsymbol{\theta}^s, \mathbf{Z}^s, K^s | \mathbf{x})}{\pi(\boldsymbol{\phi}^s, \mathbf{Y}^s, A^s, \boldsymbol{\theta}^s, \mathbf{Z}^s, K^s | \mathbf{x})} \frac{q(A^s, \mathbf{Y}^s, \boldsymbol{\phi}^s | A^s + 1, \mathbf{Y}', \boldsymbol{\phi}')}{q(A^s + 1, \mathbf{Y}', \boldsymbol{\phi}' | A^s, \mathbf{Y}^s, \boldsymbol{\phi}^s)} \frac{1}{q_{u_A}(u_A)} J_{split}^r \\ &= \frac{\pi(\boldsymbol{\phi}', \mathbf{Y}', A^s + 1, \boldsymbol{\theta}^s, \mathbf{Z}^s, K^s | \mathbf{x})}{\pi(\boldsymbol{\phi}^s, \mathbf{Y}^s, A^s, \boldsymbol{\theta}^s, \mathbf{Z}^s, K^s | \mathbf{x})} \frac{q(merge | A^s + 1)}{q(split | A^s)} \frac{q_a(a', a' + 1)}{q_a(a)} \frac{1}{q_{u_A}(u_A)} \frac{1}{q(\mathbf{Y}')} J_{split}^r, \end{aligned} \quad (\text{S.17})$$

which is the ratio of the posterior densities, the ratio of the proposal densities, and the ratio of the densities of the auxiliary variables, which is in this case just  $q_{u_A}(u_A)^{-1} = \chi_1(u_A/\sigma_A)$ , and  $J_{split}^r$  is the Jacobian. The probability of proposing a particular level to be split is simply

$$q_a(a) = \frac{1}{|\mathcal{A}^s|} = \frac{1}{A^s + 1} \forall a \in \mathcal{A}^s.$$

For the inverse merge move, see Section S:2.2.2, the probability of proposing clusters  $a'$  and  $a' + 1$  to merge is simply

$$q_a(a', a' + 1) = \frac{1}{A'} \forall a' \in \mathcal{A}' \setminus \{A'_+\},$$

therefore  $q_a(a', a' + 1)/q_a(a) = 1$ .

Let  $\mathbf{c}_a^s := \{i, \forall i \in \mathcal{I} \setminus \{1\} : \mathbf{y}_{\{i\},a}^s = 1\}$  denote the set of objects which belong to the cluster-to-be-split, i.e.,  $a$ . Then, the probability of the cluster allocation, given that cluster  $a$  has been split, is

$$q(\mathbf{Y}') = \frac{|\mathbf{c}_a^s|!}{|\mathbf{c}_{a'}^s|! |\mathbf{c}_{a'+1}^s|!} 2^{-|\mathbf{c}_a^s|}$$

since the new cluster allocations are selected at random.

Again there are three variants for both the splitting and merging of skill levels that must be considered:

#### The general case: ( $a \neq 0$ )

To preserve ordering, the same transformation is made as in Section S:2.1.1, and so the set of levels must be extended as before, but now in both positive and negative directions, such that

$$\begin{aligned} \phi_{A_+^s+1}^s &:= \phi_{A_+^s}^s + (\phi_{A_+^s}^s - \phi_{A_+^s-1}^s) \\ \phi_{A_-^s-1}^s &:= \phi_{A_-^s}^s - |\phi_{A_-^s+1}^s - \phi_{A_-^s}^s|. \end{aligned} \quad (\text{S.18})$$

Using the same logit transformation to preserve order, new skill levels are proposed via the equations

$$\phi_{a'}' = \frac{\phi_{a-1}^s + \phi_{a+1}^s \exp(-u_A) (\phi_a^s - \phi_{a-1}^s) / (\phi_{a+1}^s - \phi_a^s)}{1 + \exp(-u_A) (\phi_a^s - \phi_{a-1}^s) / (\phi_{a+1}^s - \phi_a^s)} \quad (\text{S.19})$$

$$\phi_{a'+1}' = \frac{\phi_{a-1}^s + \phi_{a+1}^s \exp(u_A) (\phi_a^s - \phi_{a-1}^s) / (\phi_{a+1}^s - \phi_a^s)}{1 + \exp(u_A) (\phi_a^s - \phi_{a-1}^s) / (\phi_{a+1}^s - \phi_a^s)}. \quad (\text{S.20})$$

where the *auxiliary variable*  $u_A \sim \sigma_A \chi_1^2$ , for  $\sigma_A > 0$ .

Combining these components, the acceptance probability of splitting skill cluster  $a$  can be computed as

$$A_{split}^r(a \neq 0) = \Lambda_{split}^r J_{split}^r, \quad (\text{S.21})$$

where

$$\Lambda_{split}^r = \frac{\pi(\boldsymbol{\phi}', \mathbf{Y}', A^s + 1, \boldsymbol{\theta}^s, \mathbf{Z}^s, K^s | \mathbf{x})}{\pi(\boldsymbol{\phi}^s, \mathbf{Y}^s, A^s, \boldsymbol{\theta}^s, \mathbf{Z}^s, K^s | \mathbf{x})} \frac{1}{1 + \mathbb{1}\{A^s = 0\}} \frac{\sigma_A}{\chi(u_A/\sigma_A)} \left( \frac{|\mathbf{c}_a^s|!}{|\mathbf{c}_{a'}^s|! |\mathbf{c}_{a'+1}^s|!} 2^{-|\mathbf{c}_a^s|} \right)^{-1}.$$

#### Splitting from the zero skill: ( $a = 0, A^s \geq 0$ )

Consider the special case that the 0 level is split, but other skill levels are present. One of the split levels must remain at 0, specifically,  $\phi_{0'}' = \phi_0^s = 0$ . The other proposed skill level is

$$\phi_{(2X-1)'}' = X\phi_{a'+1}' + (1 - X)\phi_{a'}', \quad (\text{S.22})$$

where  $X \sim \text{Bernoulli}(0.5)$ , such that the non-zero proposed skill level can be either above or below the 0 level, and it has label  $(2X - 1)'$ , that is, either  $1'$  or  $-1'$ . The Jacobian  $J_{split,0}^r$  is calculated as in Appendix S:A.3, and the acceptance probability is given as

$$A_{split}^r | (a = 0, A^s \geq 0) = 2\Lambda_{split}^r J_{split,0}^r, \quad (\text{S.23})$$

the only difference to the general case being in the Jacobian term, and the factor of 2 which comes from the Bernoulli variable.

### Splitting from the single skill model: ( $A^s = 0$ )

In the unlikely case that only a single skill level is present in the model, the new skill level is simply proposed as

$$\phi'_{(2X-1)'} = Xu_A - (1 - X)u_A, \quad (\text{S.24})$$

since no transformation is needed due to no ordering issues. In this case the acceptance probability is given as

$$A_{split}^r | (A^s = 0) = 2\Lambda_{split}^r, \quad (\text{S.25})$$

where the Jacobian term is 1.

The next state of the sampler  $(\phi^{s+1}, \mathbf{Y}^{s+1}, A^{s+1}, \theta^{s+1}, \mathbf{Z}^{s+1}, K^{s+1})$  is then accepted to be  $(\phi', \mathbf{Y}', A', \theta^s, \mathbf{Z}^s, K^s)$  with probability  $A_{split}^r$ , and otherwise  $(\phi^{s+1}, \mathbf{Y}^{s+1}, A^{s+1}, \theta^{s+1}, \mathbf{Z}^{s+1}, K^{s+1}) = (\phi^s, \mathbf{Y}^s, A^s, \theta^s, \mathbf{Z}^s, K^s)$ .

### S:2.2.2 Skill merge move

Like the intransitivity merge move, the merge move is considered as a reverse split move, such that the current parameters are  $(\phi', \mathbf{Y}', A', \theta^s, \mathbf{Z}^s, K^s) = (\phi^{s+1}, \mathbf{Y}^{s+1}, A^{s+1}, \theta^{s+1}, \mathbf{Z}^{s+1}, K^{s+1})$  be the current values of the parameters, and we aim to propose parameters  $(\phi^s, \mathbf{Y}^s, A^s, \theta^s, \mathbf{Z}^s, K^s)$ . Two levels  $a', a' + 1 \in \mathcal{A}' \setminus \{A'_+\}$  are sampled to merge with probability

$$q_a(a', a' + 1) = \frac{1}{A'} \quad \forall a' \in \mathcal{A}' \setminus \{A'_+\},$$

and are inverse split move is proposed with probability

$$q_a(a) = \frac{1}{A^s + 1} \quad \forall a \in \mathcal{A}^s \setminus \{A^s_+\},$$

so again  $q_a(a)/q_a(a', a' + 1) = 1$ . The three variants for the merging abilities are then as follows:

#### The general case: ( $a', a' + 1 \neq 0$ )

In the general case that the sampler proposed to merge two non-zero levels,  $a', a' + 1 \neq 0$ , then

$$A_{merge}^r | (a', a' + 1 \neq 0) = \Lambda_{merge}^r / J_{split}^r, \quad (\text{S.26})$$

where

$$\Lambda_{merge}^r = \frac{\pi(\phi^s, \mathbf{Y}^s, A' - 1, \theta^s, \mathbf{Z}^s, K^s | \mathbf{x})}{\pi(\phi', \mathbf{Y}', A', \theta^s, \mathbf{Z}^s, K^s | \mathbf{x})} (1 + \mathbb{1}\{A' = 1\}) \frac{\Phi(u'_A / \sigma_A)}{\sigma_A} \frac{|\mathbf{c}_a^s|!}{|\mathbf{c}_{a'}^s|! |\mathbf{c}_{a'+1}^s|!} 2^{-|\mathbf{c}_a^s|},$$

and  $u'_A \sim \sigma_A \chi_1^2$  is the value required for the inverse split move to get back to skill levels  $\phi'_{a'}$  and  $\phi'_{a'+1}$ .

**Merging to the zero skill:** ( $\min(|a'|, |a' + 1|) = 0, A' \geq 2$ )

If either  $a'$  or  $a' + 1$  are 0 (and therefore have skill levels either  $\phi'_{a'} = 0$  or  $\phi'_{a'+1} = 0$ ), then the merged skill level must be  $\phi_a = \phi_0 = 0$ , and  $u'_A$  is the value required to invert the merge, such that

$$u'_A = \begin{cases} |y(\phi'_{a'+1}|\phi'_{a'-1}, \phi'_{a'+2})| & \text{if } a' = 0 \\ |y(\phi'_{a'}|\phi'_{a'-1}, \phi'_{a'+2})| & \text{if } a' + 1 = 0 \end{cases},$$

where  $y(\cdot)$  is defined in equation (S.2). This gives an acceptance probability of

$$A_{merge}^r | [\min(|a'|, |a' + 1|) = 0, A' \geq 2] = \Lambda_{merge}^r / 2J_{split,0}^r, \quad (\text{S.27})$$

so the Jacobian  $J_{split,0}^r$ , see Appendix S:A.4, differs from the general case, and also the factor of  $1/2$ , which comes from the Bernoulli variable in the inverse split move.

**Merging to the single skill model:** ( $A' = 1$ )

If  $A' = 1$ , then the merged skill level must be 0, and  $u'_A$  is simply the absolute value of whichever level is not 0, that is  $u'_A = \max(|\phi'_{a'}|, |\phi'_{a'+1}|)$ . In this case the acceptance probability is given as

$$A_{merge}^r | (A' = 1) = \Lambda_{merge}^r / 2. \quad (\text{S.28})$$

Then, the next state is accepted to be  $(\phi^s, \mathbf{Y}^s, A^s, \theta^s, \mathbf{Z}^s, K^s) = (\phi', \mathbf{Y}', A', \theta^s, \mathbf{Z}^s, K^s)$ , with probability  $A_{merge}^r$ .

## S:3 Add-Delete components

### S:3.1 Add-Delete components : intransitivity

Empty clusters can occur after a split, if all object pairs in the split cluster move to one of the new proposed clusters. Additionally, within the Gibbs reallocation move (see Section S:4) it is possible for all object pairs in a given cluster to move to other clusters. An empty cluster could exist for a long time before being merged, and even then the proposed merge may not be accepted. To deal with this more efficiently, a *delete cluster* move is included. To satisfy detailed balance, an *add cluster* move must also be included. Define the set of empty clusters  $\mathcal{K}_e^s$  to be  $\mathcal{K}_e^s := \{a \in \{1, \dots, K^s\} : \mathbf{b}_a = \mathbf{b}_{-a} = \emptyset\}$ , such that a cluster  $k_e$  is only considered empty if both  $k_e = \emptyset$  and  $k_{-e} = \emptyset$ . This is a necessary consideration because  $\mathbf{Z}'$  was defined to contain only allocations for the ‘upper triangle’, that is  $\mathbf{Z}' := \{\mathbf{z}'_{i,j} : i > j \in \mathcal{I} \setminus \{1\}\}$ . Therefore it is possible that there are no pairs  $\{i, j\} \forall i > j \in \mathcal{I} \setminus \{1\}$  in cluster, say  $a > 0$ ; however, there may exist a pair  $\exists \{h, m\} \in -a : h > m \in \mathcal{I} \setminus \{1\}$  in cluster  $-a$ , and thus by symmetry  $\{m, h\} \in a$ . Thus, to delete a cluster  $a$ , both clusters  $a$  and  $-a$  must be empty, that is, we require  $\mathbf{b}_a = \mathbf{b}_{-a} = \emptyset$ , hence the definition of  $\mathcal{K}_e^s$ . Note also that cluster 0 is not being considered in  $\mathcal{K}_e^s$ , as there must always be exactly one transitive cluster.

#### S:3.1.1 Intransitivity add move

When a cluster is added, the proposed cluster mean  $\theta^* | \alpha, \beta \sim h_0$ , see equation (22) is drawn from the prior distribution, which is gamma distributed, and it is inserted such that correct ordering of intransitivity levels is maintained. Thus, if  $\theta^*$  is, say the  $k$ th largest value in the vector  $(\theta, \theta^*)$ , then the proposed cluster allocation changes such that  $\mathbf{b}'_l = \mathbf{b}_l^s$ ,  $\mathbf{b}'_{-l} = \mathbf{b}_{-l}^s \forall l < k$ ,  $\mathbf{b}'_{l+1} = \mathbf{b}_l^s$ ,  $\mathbf{b}'_{-(l+1)} = \mathbf{b}_{-l}^s \forall l \geq k$  and  $\mathbf{b}'_k = \mathbf{b}'_{-k} = \emptyset$ , which defines  $\mathbf{Z}'$ . The proposed intransitivity levels become  $\theta' = \{\theta_1^s, \dots, \theta_{k-1}^s, \theta^*, \theta_k^s, \dots, \theta_{k+1}^s\}$ .

The cluster allocation is then reordered by increasing the index of cluster allocations which belong to intransitivity levels which are larger than the added cluster. The probability of proposing to add a cluster is an increasing function of an algorithm parameter  $\rho_K > 0$ , and the

probability of proposing to delete a cluster, see Section S:3.1.2, is an increasing function of the current number of empty clusters,  $N_\emptyset^s := |\mathcal{K}_e^s|$ , which excludes the completely transitive set  $\mathcal{J}_T$ . Therefore, the probability of proposing to add and delete an intransitivity level is constructed as,

$$q(\text{add} \mid N_\emptyset^s) = \frac{\rho_K}{\rho_K + N_\emptyset^s}, \quad q(\text{delete} \mid N_\emptyset^s) = \frac{N_\emptyset^s}{\rho_K + N_\emptyset^s}, \quad (\text{S.29})$$

respectively.

Since an add or delete move in no way effects the likelihood, only the prior density changes, and the acceptance probability of adding is given as

$$\begin{aligned} A_{\text{add}} &= \frac{\pi(\boldsymbol{\phi}^s, \mathbf{Y}^s, A, \boldsymbol{\theta}', \mathbf{Z}', K^s + 1)}{\pi(\boldsymbol{\phi}^s, \mathbf{Y}^s, A, \boldsymbol{\theta}^s, \mathbf{Z}^s, K^s)} \frac{1}{(K^s + 1)h_0(\theta^* \mid \alpha, \beta)} \frac{(N_\emptyset^s + 1)/(\rho_K + N_\emptyset^s + 1)}{\rho_K/(\rho_K + N_\emptyset^s)} \\ &= \frac{f(\mathbf{Z}' \mid \gamma, K^s + 1)}{f(\mathbf{Z} \mid \gamma, K^s)} \frac{g_0(K^s + 1 \mid \lambda)}{g_0(K^s \mid \lambda)} \frac{(N_\emptyset^s + 1)(\rho_K + N_\emptyset^s)}{\rho_K(\rho_K + N_\emptyset^s + 1)}. \end{aligned} \quad (\text{S.30})$$

### S:3.1.2 Intransitivity delete move

During a delete empty cluster move, an empty cluster  $k_e \in \mathcal{K}_e^s$  is selected at random. Given the sampler is in state  $s$  with  $N_\emptyset^s \in \mathbb{N}_+$  empty clusters, i.e., there is at least 1 empty cluster, the acceptance probability of deleting an empty cluster,  $k_e$  with cluster mean  $\theta^*$ , where  $\mathbf{Z}'$  is the proposed allocation after the cluster is removed, is given as

$$A_{\text{delete}} = \frac{f(\mathbf{Z}' \mid \gamma, K^s - 1)}{f(\mathbf{Z}^s \mid \gamma, K^s)} \frac{g_0(K^s - 1 \mid \lambda)}{g_0(K^s \mid \lambda)} \frac{\rho_K(\rho_K + N_\emptyset^s)}{N_\emptyset^s(\rho_K + N_\emptyset^s - 1)}. \quad (\text{S.31})$$

Again, intransitivity levels are re-indexed appropriately. Choosing  $\rho_K = 1$  means that when one empty cluster exists, there is an equal chance of proposing to add or delete an empty cluster. For  $0 < \rho_K < 1$ , as long as there exists at least one cluster, there is always a greater chance of proposing to delete an empty cluster than to add an empty cluster.

### S:3.2 Add-Delete components : skills

Similarly to the add intransitivity move, for the add skill cluster move a new skill level is drawn from the prior, that is  $\phi^* \mid \nu_A \sim \mathcal{N}(0, \nu_A^2)$ , and indexed such that the proposed vector of skill levels is ordered. The allocations are altered such that all objects maintain the same abilities.

Define the set of empty skill clusters  $\mathcal{A}_e^s$  to be  $\mathcal{A}_e^s := \{a \in \mathcal{A}_{-0} : \mathbf{c}_a = \emptyset\}$ , noting that cluster 0 is not being considered. During a delete empty cluster move, an empty cluster, say  $a_e \in \mathcal{A}_e^s$ , is selected at random to be deleted. The cluster allocations are then reordered such that, if the deleted level is positive, the index of cluster allocations which belong to skill levels which are larger than the removed cluster are decreased by one, and if the deleted level is negative, the index of cluster allocations which belong to skill levels which are smaller than the removed cluster are increased by one. That is,  $\mathbf{c}'_l = \mathbf{c}_l^s - 1$  if  $l > \max(a_e, 0)$ ,  $\mathbf{c}'_l = \mathbf{c}_l^s + 1$  if  $l < \min(a_e, 0)$  and  $\mathbf{c}'_l = \mathbf{c}_l^s$  otherwise. Similarly to the intransitivity add and delete moves, the probability of proposing a skill cluster is an increasing function of an algorithm parameter  $\rho_A > 0$ , and the probability of proposing to delete a cluster is increasing function of the current number of empty clusters,  $N_{\emptyset_A}^s := |\mathcal{A}_e^s|$ . The probability of proposing to add or delete an empty skill cluster is, respectively,

$$q(\text{add } A \mid N_{\emptyset_A}^s) = \frac{\rho_A}{\rho_A + N_{\emptyset_A}^s}, \quad q(\text{delete } A \mid N_{\emptyset_A}^s) = \frac{N_{\emptyset_A}^s}{\rho_A + N_{\emptyset_A}^s}. \quad (\text{S.32})$$

Given the sampler is in state  $s$  with  $N_{\emptyset_A}^s \in \mathbb{N}$  empty clusters, the acceptance probability of adding is given as

$$A_{add\ A} = \frac{f(\mathbf{Y}'|\gamma_A, A^s + 1)}{f(\mathbf{Y}|\gamma_A, A^s)} \frac{g_0(A^s + 1|\lambda_A)}{g_0(A^s|\lambda_A)} \frac{(N_{\emptyset_A}^s + 1)(\rho_A + N_{\emptyset_A}^s)}{\rho_A(\rho_A + N_{\emptyset_A}^s + 1)}. \quad (\text{S.33})$$

Likewise, given the sampler is in state  $s$  with  $N_{\emptyset_A}^s \in \mathbb{N}_+$  empty clusters, the acceptance probability of deleting an empty cluster,  $a$  with cluster mean  $\phi^*$ , where  $\mathbf{Y}'$  is the proposed allocation after the cluster is removed, is given as

$$A_{delete\ A} = \frac{f(\mathbf{Y}'|\gamma_A, A^s - 1)}{f(\mathbf{Y}|\gamma_A, A^s)} \frac{g_0(A^s - 1|\lambda_A)}{g_0(A^s|\lambda_A)} \frac{\rho_A(\rho_A + N_{\emptyset_A}^s)}{N_{\emptyset_A}^s(\rho_A + N_{\emptyset_A}^s - 1)}. \quad (\text{S.34})$$

## S:4 Standard MCMC updates

### S:4.1 Standard MCMC updates : intransitivity

#### S:4.1.1 Intransitivity levels update

Moves which do not propose any change to  $K^s$  or  $A^s$  can follow standard MCMC updates. The moves follow a Metropolis-Hastings-within-Gibbs procedure, where the skill levels  $\phi$ , intransitivity levels  $\theta$ , and cluster allocations  $(\mathbf{Y}, \mathbf{Z})$  are updated sequentially.

The intransitivity levels are updated sequentially from smallest to largest, using the matching function (S.2) to ensure ordering is preserved. First, the proposed transformed intransitivity level  $y(\theta'_1|\theta_0^s, \theta_2^s)$  is proposed via a symmetric random walk with standard deviation  $\tau > 0$ , such that  $y(\theta'_1|\theta_0^s, \theta_2^s) \sim \mathcal{N}(y(\theta_1^s|\theta_0^s, \theta_2^s), \tau^2)$ , and accepted with probability  $A_{levels}^{(1)}$ , where

$$A_{levels}^{(1)} = \frac{\pi(\phi^s, \mathbf{Y}^s, A^s, \theta', \mathbf{Z}^s, K^s|\mathbf{x})}{\pi(\phi^s, \mathbf{Y}^s, A^s, \theta^s, \mathbf{Z}^s, K^s|\mathbf{x})} = \frac{L(\mathbf{x}|\phi^s, \mathbf{Y}^s, A^s, \theta', \mathbf{Z}^s, K^s)}{L(\mathbf{x}|\phi^s, \mathbf{Y}^s, A^s, \theta^s, \mathbf{Z}^s, K^s)} \frac{h_0(\theta'_1|\alpha, \beta)}{h_0(\theta_1^s|\alpha, \beta)}. \quad (\text{S.35})$$

and if accepted then  $\theta_1^{s+1} = \theta'_1$ . The other intransitivity levels are then drawn similarly, but using the latest updated values of the intransitivity levels, such that

$$y(\theta'_k|\theta_{k-1}^{s+1}, \theta_{k+1}^s) \sim \mathcal{N}(y(\theta_k^s|\theta_{k-1}^{s+1}, \theta_{k+1}^s), \tau^2),$$

and  $\theta'_k$  is accepted as the new parameter value  $\theta_k^{s+1}$  with probability  $A_{levels}^{(k)}$ , where

$$A_{levels}^{(k)} = \frac{\pi(\phi^s, \mathbf{Y}^s, A^s, \theta'_k, \mathbf{Z}^s, K^s|\mathbf{x})}{\pi(\phi^s, \mathbf{Y}^s, A^s, \theta_k^s, \mathbf{Z}^s, K^s|\mathbf{x})} = \frac{L(\mathbf{x}|\phi^s, \mathbf{Y}^s, A^s, \theta'_k, \mathbf{Z}^s, K^s)}{L(\mathbf{x}|\phi^s, \mathbf{Y}^s, A^s, \theta_k^s, \mathbf{Z}^s, K^s)} \frac{h_0(\theta'_k|\alpha, \beta)}{h_0(\theta_k^s|\alpha, \beta)}, \quad (\text{S.36})$$

where  $\theta_k^s := \{\theta_1^{s+1}, \dots, \theta_{k-1}^{s+1}, \theta_k^s, \dots, \theta_{K^s}^s\}$  and  $\theta'_k := \{\theta_1^{s+1}, \dots, \theta_{k-1}^{s+1}, \theta'_k, \theta_{k+1}^s, \dots, \theta_{K^s}^s\}$ .

#### S:4.1.2 Pair reallocation

Then the intransitivity cluster allocation  $\mathbf{Z}$  is updated. This can be achieved by either a naïve approach, or using the conditional posterior approach. For the naïve approach, a new allocation is drawn from the prior  $f(\mathbf{Z}|\gamma, K)$ , using a two-step process. First, a new  $\omega'_{K^s}$  is drawn from the prior  $\omega'_{K^s}|K^s \sim \text{Dirichlet}(\gamma \mathbf{1}_{2K+1})$ . Then, the allocations are drawn from

$$\mathbf{Z}' = \{z'_{\{i,j\}}|\omega'_{K^s} \sim \text{multinomial}(1, \omega'_{K^s}), \forall i > j \in \mathcal{I} \setminus \{1\}\},$$

with  $z'_{\{i,j\}} \perp z'_{\{h,m\}}|\omega'_{K^s}$  for all  $\{i,j\} \neq \{h,m\} \in (\mathcal{I} \setminus \{1\})^2$ , and so by mixing over  $\omega'_{K^s}$  we are sampling from  $f(\mathbf{Z}|\gamma, K)$ . This will be fast, but may mix over iterations poorly since the proposal could be far away from the maximum posterior and so the acceptance rate could be very low.

Instead, the data can be used to inform the next proposal using the conditional posterior. Consider the pair  $\{i, j\} : i > j \in \mathcal{I} \setminus \{1\}$  at step  $s$ . The conditional posterior  $p_{\{i,j\}}^s(y)$  that the pair  $\{i, j\}$  is in cluster  $y \in \{-K^s, \dots, K^s\}$  is computed as

$$p_{\{i,j\}}^s(y) \propto L(\mathbf{x}_{\{i,j\}} | \boldsymbol{\phi}^s, \mathbf{Y}^s, A^s, \boldsymbol{\theta}^s, \tilde{\mathbf{z}}_{\{i,j\}}(y), K^s) f(\tilde{\mathbf{Z}}_{\{i,j\}}^s(y) | \gamma, K^s), \quad \forall y \in \{-K^s, \dots, K^s\}, \quad (\text{S.37})$$

for all  $i > j \in \mathcal{I} \setminus \{1\}$ , where  $\tilde{\mathbf{z}}_{\{i,j\}}(y)$  indicates that the pair  $\{i, j\}$  is in cluster  $y$ , i.e.,

$$\tilde{\mathbf{z}}_{\{i,j\}}(y) := \{z_t, t \in \{-K^s, \dots, K^s\} : z_y = 1, z_t = 0 \text{ otherwise}\},$$

and  $\mathbf{x}_{\{i,j\}}$  comprises only data of comparisons between  $i$  and  $j$ , and the full allocations used in the prior  $f(\tilde{\mathbf{Z}}_{\{i,j\}}^s(y) | \gamma, K^s)$  are given as

$$\tilde{\mathbf{Z}}_{\{i,j\}}^s(y) = \{\tilde{\mathbf{z}}_{\{i,j\}}(y), \{\mathbf{z}_{\{a,b\}}^s, \forall a > b \in \mathcal{I} \setminus \{1, i, j\}\}\},$$

which is just the usual set of allocations, except for the pair  $\{i, j\}$ , which is assigned to cluster  $y$ . Only the data  $\mathbf{x}_{\{i,j\}}$  need be considered in the likelihood in equation (S.40) instead of the all the data, because the cluster allocation of all pairs is assumed to be independent, so only  $\theta_{ik}$  will change, see definition (12), which in turn means that only the pairwise probabilities  $p_{ik}$  and  $p_{ki}$  will change, see equation (7).

Since  $K^s$  is finite, for all  $s \in \{1, \dots, S\}$ , the probability  $q_{\{i,j\}}^s(y)$  at iteration  $s$  that the pair  $\{i, j\}$  belongs to a cluster  $y$  is found by simply normalising, to give

$$q_{\{i,j\}}^s(y) := \frac{p_{\{i,j\}}^s(y)}{\sum_{c=-K^s}^{K^s} p_{\{i,j\}}^s(c)}, \quad \forall y \in \{-K^s, \dots, K^s\}.$$

Then, for the pair  $\{i, j\}$ , the proposed allocation is drawn from a multinomial distribution with probability  $\mathbf{q}_{\{i,j\}}^s := \{q_{\{i,j\}}^s(y) : y \in \{-K^s, \dots, K^s\}\}$ , so that

$$\mathbf{z}'_{\{i,j\}} \sim \text{multinomial}\left(1, \mathbf{q}_{\{i,j\}}^s\right). \quad (\text{S.38})$$

Note that it is possible for  $\mathbf{z}'_{\{i,j\}} = \mathbf{z}_{\{i,j\}}^s$ .

So far we have explained the proposal for a given pair  $\{i, j\}$ . In order to reallocate all pairs, this proposal is made sequentially for all  $i > j \in \mathcal{I} \setminus \{1\}$  as follows. All free pairs are initially placed into a *holding set*  $\mathcal{H} = \{\{a, b\} : a > b \in \mathcal{I} \setminus \{1\}\}$ . Also define an *allocated set*  $\mathcal{L}$  which is initially empty. From the holding set  $\mathcal{H}$ , a pair  $\{i, j\} \in \mathcal{H}$  is selected at random to have a new allocation proposed  $\mathbf{z}'_{\{i,j\}}$ , which is drawn from equation (S.38). This is then accepted with probability  $A_{\text{alloc}}^{\{i,j\}} = 1, \forall \{i, j\} : i > j \in \mathcal{I} \setminus \{1\}$ , see appendix S:B. Therefore  $\mathbf{z}_{\{i,j\}}^{s+1} = \mathbf{z}'_{\{i,j\}}$  with probability 1 for all  $i > j \in \mathcal{I}$ . Then, the pair  $\{i, j\}$  are placed in the allocated set, such that now  $\mathcal{H} = \{\{a, b\} : a > b \in (\mathcal{I} \setminus \{1\})^2 \setminus \{i, j\}\}$ , and the allocated set becomes  $\mathcal{L} = \{\{i, j\}\}$ . Pairs from the holding set continue to be reallocated until the holding set is empty, and all pairs have been reassigned.

## S:4.2 Standard MCMC updates : skills

### S:4.2.1 Skill levels update

Next the skill levels are updated sequentially from smallest to largest, and the new values are again proposed on the transformed scale, all of which ensures that order is preserved. Specifically, for any  $a \in \mathcal{A}_{\{-0\}}$ , then the new transformed parameter is proposed via a symmetric random walk with standard deviation  $\tau_A > 0$ , such that  $y(\phi'_a | \phi_{a-1}^{s+1}, \phi_{a+1}^s) \sim \mathcal{N}(y(\phi_a^s | \phi_{a-1}^{s+1}, \phi_{a+1}^s), \tau_A^2)$ . The proposed parameter is accepted with probability

$$A_{\text{levels}}^{(a)} = \frac{\pi(\boldsymbol{\phi}', \mathbf{Y}^s, A^s, \boldsymbol{\theta}^s, \mathbf{Z}^s, K^s | \mathbf{x})}{\pi(\boldsymbol{\phi}^s, \mathbf{Y}^s, A^s, \boldsymbol{\theta}^s, \mathbf{Z}^s, K^s | \mathbf{x})} = \frac{L(\mathbf{x} | \boldsymbol{\phi}', \mathbf{Y}^s, A^s, \boldsymbol{\theta}^s, \mathbf{Z}^s, K^s)}{L(\mathbf{x} | \boldsymbol{\phi}^s, \mathbf{Y}^s, A^s, \boldsymbol{\theta}^s, \mathbf{Z}^s, K^s)} \frac{\pi(\phi'_a | \nu_A)}{\pi(\phi_a^s | \nu_A)}. \quad (\text{S.39})$$

where  $\pi$  is the prior distribution of the skill levels  $\boldsymbol{\phi}$ , namely, normal with standard deviation  $\nu_A$ . If accepted then  $\phi_a^{s+1} = \phi'_a$ .

### S:4.2.2 Object reallocation

The skill cluster allocation is updated in the same way as the intransitivity cluster allocation, using the conditional posterior. By considering the object  $i \in \mathcal{I} \setminus \{1\}$  at step  $s$ , the conditional posterior  $p_{\{i\}}^s(w)$  that the object  $i$  is in cluster  $w \in \{-A_-^s, \dots, A_+^s\}$  is

$$p_{\{i\}}^s(w) \propto L(\mathbf{x}_{\{i\}} | \boldsymbol{\phi}^s, \tilde{\mathbf{Y}}_{\{i\}}(w), A^s, \boldsymbol{\theta}^s, \mathbf{Z}^s, K^s) f(\tilde{\mathbf{Y}}_{\{i\}}^s(w) | \gamma_A, A^s), \quad \forall y \in \{-A_-^s, \dots, A_+^s\}, \quad i \in \mathcal{I} \setminus \{1\} \quad (\text{S.40})$$

where

$$\tilde{\mathbf{Y}}_{\{i\}}^s(w) := \{\tilde{\mathbf{y}}_{\{i\}}(w), \{\mathbf{y}_{\{i\}}^s, \forall i \in \mathcal{I} \setminus \{1, i\}\}\},$$

and  $\tilde{\mathbf{y}}_{\{i\}}(w)$  indicates that object  $i$  is in cluster  $w$ , i.e.,

$$\tilde{\mathbf{y}}_{\{i\}}(w) := \{y_t, t \in \{-A_-^s, \dots, A_+^s\} : y_w = 1, y_t = 0 \text{ otherwise}\}.$$

Here,  $\mathbf{x}_{\{i\}}$  are only the data involving comparisons with object  $i$ , which is possible because all skill cluster allocations and skill clusters are assumed to be independent and so the likelihood of comparisons not involving object  $i$  will not be effected.

The probability  $q_{\{i\}}^s(w)$  at iteration  $s$  that the object  $i$  belongs to a cluster  $w$  is again found by normalising, to give

$$q_{\{i\}}^s(w) := \frac{p_{\{i\}}^s(w)}{\sum_{c=-A_-^s}^{A_+^s} p_{\{i\}}^s(c)}, \quad \forall w \in \{-A_-^s, \dots, A_+^s\}, \quad \forall i \in \mathcal{I} \setminus \{1\}.$$

Then the object  $i$ 's the proposed allocation is drawn from a multinomial distribution with probability  $\mathbf{q}_{\{i\}}^s := \{q_{\{i\}}^s(w) : w \in \{-A_-^s, \dots, A_+^s\}\}$ , so that

$$\mathbf{y}'_{\{i\}} \sim \text{multinomial}\left(1, \mathbf{q}_{\{i\}}^s\right), \quad \forall i \in \mathcal{I} \setminus \{1\}. \quad (\text{S.41})$$

Note that it is possible for  $\mathbf{y}'_{\{i\}} = \mathbf{y}_{\{i\}}^s$ . Again, the full proposal for all objects is made sequentially for all  $i \in \mathcal{I} \setminus \{1\}$  as follows. All objects, except for the fixed object 1, are initially placed into a *holding set*  $\mathcal{H}_A = \{i : i \in \mathcal{I} \setminus \{1\}\}$ . Also define an *allocated set*  $\mathcal{L}_A = \emptyset$ . From the holding set  $\mathcal{H}_A$ , an object  $i \in \mathcal{H}_A$  is selected at random to have a new allocation proposed  $\mathbf{y}'_{\{i\}}$ , which is drawn from equation (S.41). This is then accepted with probability  $A_{alloc}^{\{i\}} = 1, \forall \{i\} : i \in \mathcal{I} \setminus \{1\}$ , see appendix S:B. The object  $i$  is then placed in the allocated set, such that now  $\mathcal{H}_A = \{i : i \in \mathcal{I} \setminus \{1, i\}\}$ , and the allocated set becomes  $\mathcal{L}_A = \{i\}$ . Objects from the holding set continue to be reallocated until the holding set is empty.

## S:5 Initialisation

To ensure the best possible chance of convergence of the RJMCMC algorithm, good initial parameter estimates are useful. The full initialisation routine is described in algorithm 1. A standard Bradley-Terry model is first fitted to the data, which gives the abilities  $\{r_i^{(BT)} : i \in \mathcal{I}\}$ , and the associated pairwise win probabilities  $\{p_{ik}^{(BT)} : i > k \in \mathcal{I} \setminus \{1\}\}$ . Then, from the data, if  $w_{ik}$  is the number of comparisons in which object  $i$  is favoured to object  $k$ , out of a possible  $n_{ik}$  comparisons, then a set of naive pairwise probabilities can be formed by using these, and regularised with a prior. If  $\{p_{ik}^{(n)} := w_{ik}/n_{ik} : i > k \in \mathcal{I} \setminus \{1\}\}$ , which can be considered as  $w_{ik} \sim \text{Binomial}(n_{ik}, p_{ik}^{(n)})$ , then by using a beta prior  $\bar{p} \sim \text{Beta}(\alpha_p, \beta_p)$ ,  $\alpha_p, \beta_p > 0$ , the initial naive posterior probabilities are set to

$$\left\{ \hat{p}_{ik}^{(n)} = \left( \frac{w_{ik} + \alpha_p}{n_{ik} + \alpha_p + \beta_p} \right) : i > k \in \mathcal{I} \setminus \{1\} \right\}.$$

This regularisation prevents values of  $\hat{p}_{ik}^{(n)}$  becoming too close to, or exactly, 0 or 1, which result in unrealistic and therefore poor starting values for the intransitivity. This is no concern in the main RJMCMC algorithm because the prior helps to regularise this. From these two sets of probabilities, the initial estimates for the intransitivity are found as

$$\left\{ \theta_{ik} = \log \left( \frac{\hat{p}_{ik}^{(n)} / (1 - \hat{p}_{ik}^{(n)})}{p_{ik}^{(BT)} / (1 - p_{ik}^{(BT)})} \right) : i > k \in \mathcal{I} \setminus \{1\} \right\}.$$

These values of intransitivity are clustered into their initial levels  $\boldsymbol{\theta}$  using  $k$ -means clustering. This is done across a range of number of levels  $K$  to produce several separate initial models. The BIC is then calculated for each model, and the best is returned. Conditional on this model, the abilities  $\mathbf{r}^{(BT)}$  are also clustered again by using several  $k$ -means algorithms across a range of  $A$ , and the best model according to the BIC is selected as the initial estimates for the ICBT model.

Instead of applying the full RJMCMC algorithm to this initial model, initially only the skill levels  $\boldsymbol{\phi}$  and the intransitivity levels  $\boldsymbol{\theta}$  are permitted to update, with the other parameters  $(\mathbf{Z}, \mathbf{Y}, K, A)$  fixed. After convergence of this algorithm, a second MCMC algorithm then allows additionally the allocations  $\mathbf{Y}$  and  $\mathbf{Z}$  to update. Finally, only after convergence of these two MCMC algorithms, is the full split-merge RJMCMC algorithm implemented, where samples are taken from all of  $(\boldsymbol{\theta}, \boldsymbol{\phi}, \mathbf{Z}, \mathbf{Y}, K, A)$ . The full algorithm, including all the initialisation is detailed in Algorithm 1.

---

**Algorithm 1:** Reversible Jump algorithm for Clustered Intransitive Bradley-Terry model.

---

Inputs: paired comparison data, prior parameters  $(\lambda, \lambda_A \gamma, \gamma_A, \alpha, \beta)$ ;  
Find maximum likelihood estimates for the Bradley-Terry abilities  $\{r_i : i \in \mathcal{I}\}$ , and the associated pairwise probabilities  $\{p_{ik}^{(BT)} : i \neq k \in \mathcal{I}\}$ ;  
Find naive estimates for pairwise win probabilities  $\{p_{ik}^{(n)} = w_{ik}/n_{ik} : i \neq k \in \mathcal{I}\}$ ;  
Find initial estimates for intransitivity

$$\left\{ \theta_{ik} = \log \left( \frac{p_{ik}^{(n)} / (1 - p_{ik}^{(n)})}{p_{ik}^{(BT)} / (1 - p_{ik}^{(BT)})} \right) : i \neq k \in \mathcal{I} \right\};$$

Cluster into intransitivity levels and skill levels using  $k$ -means clustering. Pick model with best BIC as initial model, which gives initial parameter estimates  $(\hat{\phi}_{\text{initial}}, \hat{\mathbf{Y}}_{\text{initial}}, A_{\text{initial}}, \hat{\mathbf{Z}}_{\text{initial}}, \hat{\boldsymbol{\theta}}_{\text{initial}}, K_{\text{initial}})$ ;

Set  $(\phi^0, \mathbf{Y}^0, A^0, \boldsymbol{\theta}^0, \mathbf{Z}^0, K^0) = (\hat{\phi}_{\text{initial}}, \hat{\mathbf{Y}}_{\text{initial}}, A_{\text{initial}}, \hat{\mathbf{Z}}_{\text{initial}}, \hat{\boldsymbol{\theta}}_{\text{initial}}, K_{\text{initial}})$ ;

**for**  $s = 1, \dots, S_1$ , **do**

    Update  $\boldsymbol{\theta}$ ;  
    Update  $\phi$ ;  
    Store sample  $(\phi^s, \mathbf{Y}^s, A^s, \boldsymbol{\theta}^s, \mathbf{Z}^s, K^s)$

**end**

Set  $(\phi^0, \mathbf{Y}^0, A^0, \boldsymbol{\theta}^0, \mathbf{Z}^0, K^0) = \arg\max_s \pi(\phi^s, \mathbf{Y}^s, A^s, \boldsymbol{\theta}^s, \mathbf{Z}^s, K^s | \mathbf{x})$

**for**  $s = 1, \dots, S_2$ , **do**

    Update  $\boldsymbol{\theta}$ ;  
    Update  $\mathbf{Z}$ ;  
    Update  $\phi$ ;  
    Update  $\mathbf{Y}$ ;  
    Store sample  $(\phi^s, \mathbf{Y}^s, A^s, \boldsymbol{\theta}^s, \mathbf{Z}^s, K^s)$

**end**

Set  $(\phi^0, \mathbf{Y}^0, A^0, \boldsymbol{\theta}^0, \mathbf{Z}^0, K^0) = \arg\max_s \pi(\phi^s, \mathbf{Y}^s, A^s, \boldsymbol{\theta}^s, \mathbf{Z}^s, K^s | \mathbf{x})$

**for**  $s = 1, \dots, S$ , **do**

    Update  $\boldsymbol{\theta}$ ;  
    Update  $\phi$ ;  
    Let  $K^s = K^{s-1}, A^s = A^{s-1}$ ;  
    **if**  $K^s = 1$  **then**  
        | propose to split an intransitivity cluster;  
    **else**  
        | with probability 1/2 propose to split or merge an intransitivity cluster;  
    **end**  
    **if** *there are no empty intransitivity clusters* **then**  
        | propose adding empty intransitivity cluster  
    **else**  
        | with probability  $\frac{N_\emptyset}{N_\emptyset + \rho_K}$  propose deleting empty intransitivity cluster;  
        **or**;  
        | with probability  $\frac{\rho_K}{N_\emptyset + \rho_K}$  propose adding intransitivity empty cluster;  
    **end**  
    **if**  $A^s = 1$  **then**  
        | propose to split a skill level  
    **else**  
        | with probability 1/2 propose to split or merge a skill level;  
    **end**  
    **if** *there are no empty skill clusters* **then**  
        | propose adding empty skill cluster  
    **else**  
        | with probability  $\frac{N_\emptyset}{N_\emptyset + \rho_A}$  propose deleting empty skill cluster;  
        **or**;  
        | with probability  $\frac{\rho_A}{N_\emptyset + \rho_A}$  propose adding empty skill cluster;  
    **end**  
    Update  $\mathbf{Z}$ ;  
    Update  $\mathbf{Y}$ ;  
    Store sample  $(\phi^s, \mathbf{Y}^s, A, \boldsymbol{\theta}^s, \mathbf{Z}^s, K^s)$

**end**

# Appendices

## S:A Jacobian Calculations for Split and Merge Moves

### S:A.1 Jacobian for intransitivity split move: $k \neq 0$

The Jacobian for the intransitivity split move  $J_{split}$ , for the general case where  $k \neq 0$ , namely, not a split on the transitive cluster, is given as

$$J_{split} = \begin{vmatrix} \frac{\partial \theta'_{k'+1}}{\partial \theta_k} & \frac{\partial \theta'_{k'}}{\partial \theta_k} \\ \frac{\partial \theta'_{k'+1}}{\partial u} & \frac{\partial \theta'_{k'}}{\partial u} \end{vmatrix}.$$

Let  $\alpha = \theta_{k-1}$ ,  $\beta = \theta_{k+1}$ . From equations (S.5) and (S.6), we have

$$\begin{aligned} \theta'_{k'} &= \frac{\alpha + \beta \exp(-u) (\theta_k - \alpha) / (\beta - \theta_k)}{1 + \exp(-u) (\theta_k - \alpha) / (\beta - \theta_k)} \\ \theta'_{k'+1} &= \frac{\alpha + \beta \exp(u) (\theta_k - \alpha) / (\beta - \theta_k)}{1 + \exp(u) (\theta_k - \alpha) / (\beta - \theta_k)}. \end{aligned}$$

Therefore, using the quotient rule twice,

$$\begin{aligned} \frac{\partial \theta'_{k'}}{\partial \theta_k} &= \frac{\left[1 + \exp(-u) \left(\frac{\theta_k - \alpha}{\beta - \theta_k}\right)\right] \beta \exp(-u) \frac{\beta - \alpha}{(\beta - \theta_k)^2} - \left[\alpha + \beta \exp(-u) \left(\frac{\theta_k - \alpha}{\beta - \theta_k}\right)\right] \exp(-u) \frac{\beta - \alpha}{(\beta - \theta_k)^2}}{\left[1 + \exp(-u) \left(\frac{\theta_k - \alpha}{\beta - \theta_k}\right)\right]^2} \\ &= \frac{\beta \exp(-u) \frac{\beta - \alpha}{(\beta - \theta_k)^2} \left[1 - \frac{\alpha}{\beta}\right]}{\left[1 + \exp(-u) \left(\frac{\theta_k - \alpha}{\beta - \theta_k}\right)\right]^2}, \end{aligned} \quad (\text{S.42})$$

and similarly

$$\frac{\partial \theta'_{k'+1}}{\partial \theta_k} = \frac{\beta \exp(u) \frac{\beta - \alpha}{(\beta - \theta_k)^2} \left[1 - \frac{\alpha}{\beta}\right]}{\left[1 + \exp(u) \left(\frac{\theta_k - \alpha}{\beta - \theta_k}\right)\right]^2}, \quad (\text{S.43})$$

$$\begin{aligned} \frac{\partial \theta'_{k'}}{\partial u} &= \frac{\left[1 + \exp(-u) \left(\frac{\theta_k - \alpha}{\beta - \theta_k}\right)\right] \beta \exp(-u) (-1) \frac{\theta_k - \alpha}{\beta - \theta_k} - \left[\alpha + \beta \exp(-u) \left(\frac{\theta_k - \alpha}{\beta - \theta_k}\right)\right] \exp(-u) (-1) \frac{\theta_k - \alpha}{\beta - \theta_k}}{\left[1 + \exp(-u) \left(\frac{\theta_k - \alpha}{\beta - \theta_k}\right)\right]^2} \\ &= - \frac{\beta \exp(-u) \frac{\theta_k - \alpha}{\beta - \theta_k} \left[1 - \frac{\alpha}{\beta}\right]}{\left[1 + \exp(-u) \left(\frac{\theta_k - \alpha}{\beta - \theta_k}\right)\right]^2}, \end{aligned} \quad (\text{S.44})$$

$$\frac{\partial \theta'_{k'+1}}{\partial u} = \frac{\beta \exp(u) \frac{\theta_k - \alpha}{\beta - \theta_k} \left[1 - \frac{\alpha}{\beta}\right]}{\left[1 + \exp(u) \left(\frac{\theta_k - \alpha}{\beta - \theta_k}\right)\right]^2}. \quad (\text{S.45})$$

Equations (S.42), (S.43), (S.44), (S.45) therefore give a Jacobian of

$$\begin{aligned} J_{split} &= \left| \frac{\beta \exp(u) \frac{\beta - \alpha}{(\beta - \theta_k)^2} \left[1 - \frac{\alpha}{\beta}\right] (-1) \beta \exp(-u) \frac{\theta_k - \alpha}{\beta - \theta_k} \left[1 - \frac{\alpha}{\beta}\right] - \beta \exp(-u) \frac{\beta - \alpha}{(\beta - \theta_k)^2} \left[1 - \frac{\alpha}{\beta}\right] \beta \exp(u) \frac{\theta_k - \alpha}{\beta - \theta_k} \left[1 - \frac{\alpha}{\beta}\right]}{\left[1 + \exp(u) \left(\frac{\theta_k - \alpha}{\beta - \theta_k}\right)\right]^2 \left[1 + \exp(-u) \left(\frac{\theta_k - \alpha}{\beta - \theta_k}\right)\right]^2} \right| \\ &= \frac{2\beta^2 \frac{(\beta - \alpha)(\theta_k - \alpha)}{(\beta - \theta_k)^3} \left[1 - \frac{\alpha}{\beta}\right]^2}{1 + 4 \cosh(u) \left(\frac{\theta_k - \alpha}{\beta - \theta_k}\right) + (4 + 2 \cosh(2u)) \left(\frac{\theta_k - \alpha}{\beta - \theta_k}\right)^2 + 4 \cosh(u) \left(\frac{\theta_k - \alpha}{\beta - \theta_k}\right)^3 + \left(\frac{\theta_k - \alpha}{\beta - \theta_k}\right)^4}, \end{aligned} \quad (\text{S.46})$$

and  $J_{merge} = 1/J_{split}$ .

### S:A.2 Jacobian for skill split move: $a \neq 0$

For the corresponding split of a skill cluster, assuming it is not the 0 cluster, i.e.,  $a \neq 0$ , let  $\alpha = \phi_{a-1}$ ,  $\beta = \phi_{a+1}$ . Then similarly to Appendix S:A.1, the Jacobian for the general split move for the skill levels is given as,

$$J_{split}^A = \frac{2\beta^2 \frac{(\beta-\alpha)(\phi_a-\alpha)}{(\beta-\phi_a)^3} \left[1 - \frac{\alpha}{\beta}\right]^2}{1 + 4 \cosh(u_A) \left(\frac{\phi_a-\alpha}{\beta-\phi_a}\right) + (4 + 2 \cosh(2u_A)) \left(\frac{\phi_a-\alpha}{\beta-\phi_a}\right)^2 + 4 \cosh(u_A) \left(\frac{\phi_a-\alpha}{\beta-\phi_a}\right)^3 + \left(\frac{\phi_a-\alpha}{\beta-\phi_a}\right)^4}, \quad (\text{S.47})$$

where  $J_{merge}^A = 1/J_{split}^A$ .

### S:A.3 Jacobian for intransitivity split move: $k = 0$

In the case that the transitive level has a split proposed, i.e.,  $k = 0$ , then

$$\theta'_{k'} = \theta_k = \theta_0 = 0,$$

and so

$$\frac{\partial \theta'_{k'}}{\partial u} = 0, \quad \frac{\partial \theta'_k}{\partial \theta_k} = 1.$$

Therefore, with  $\alpha$  and  $\beta$  defined as in Appendix S:A.1, the Jacobian is given as

$$\begin{aligned} J_{split}|(k=0) &= \left| \frac{\partial \theta'_{k'+1}}{\partial u} \right| |(k=0)| \\ &= \frac{\beta \exp(u) \frac{\theta_0-\alpha}{(\beta-\theta_0)^2} \left[1 - \frac{\alpha}{\beta}\right]}{\left[1 + \exp(u) \left(\frac{\theta_0-\alpha}{\beta-\theta_0}\right)\right]^2} \\ &= \frac{2\beta \exp(u)}{(1 + \exp(u))^2}, \end{aligned} \quad (\text{S.48})$$

where the last equality follows since  $\alpha = -\beta$ .

### S:A.4 Jacobian for skill split move: $a = 0$

The Jacobian here is derived very similarly to Appendix S:A.3, except that, since the levels can be negative and are not reflected around 0, it is not necessarily true that  $\alpha = -\beta$ . Moreover, if a split occurs on cluster  $a$  with  $\phi_a = 0$ , then either  $\phi'_{a'} = 0$  or  $\phi'_{a'+1} = 0$ , with equal probability, as explained in the algorithm. In the case that  $\phi'_{a'} = 0$ , then

$$\phi'_{a'} = \phi_a = \phi_0 = 0,$$

and

$$\frac{\partial \phi'_{a'}}{\partial u} = 0, \quad \frac{\partial \phi'_{a'}}{\partial \phi_a} = 1.$$

Therefore the Jacobian is given as

$$\begin{aligned} J_{split}|(a=0) &= \left| \frac{\partial \phi'_{a'+1}}{\partial u} \right| \\ &= \frac{\exp(u) \frac{-\alpha}{\beta} \left[1 - \frac{\alpha}{\beta}\right]}{\left[1 + \exp(u) \left(\frac{-\alpha}{\beta}\right)\right]^2} \end{aligned} \quad (\text{S.49})$$

However, if  $\phi'_{a'+1} = 0$ , then  $\phi'_{a'+1} = \phi_a = \phi_0 = 0$ , which leads to the same result.

## S:B Allocation acceptance probability

The probability of accepting the proposed allocation for a pair  $\{i, j\}$ , is

$$A_{alloc}^{\{i,j\}} = \frac{L(\mathbf{x}_{\{i,j\}}|\boldsymbol{\phi}^s, \mathbf{Y}^s, A^s, \boldsymbol{\theta}^s, \mathbf{z}'_{\{i,j\}}, K^s) f(\mathbf{Z}'|\gamma, K^s) q_z(\mathbf{Z}^s|\mathbf{q}_{\{i,j\}}^s)}{L(\mathbf{x}_{\{i,j\}}|\boldsymbol{\phi}^s, \mathbf{Y}^s, A^s, \boldsymbol{\theta}^s, \mathbf{z}_{\{i,j\}}^s, K^s) f(\mathbf{Z}^s|\gamma, K^s) q_z(\mathbf{Z}'|\mathbf{q}_{\{i,j\}}^s)}, \quad (\text{S.50})$$

where

$$\mathbf{Z}' = \{\mathbf{z}'_{\{i,j\}}, \{\mathbf{z}_{\{h\}}^s : h \in \mathcal{H}\}, \{\mathbf{z}_{\{l\}}^{s+1} : l \in \mathcal{L}\}\},$$

is the set comprising the proposed allocation, the allocations from pairs in the holding set, and the new allocations of any pairs in the allocated set, and

$$\frac{q_z(\mathbf{Z}^s|\mathbf{q}_{\{i,j\}}')}{q_z(\mathbf{Z}'|\mathbf{q}_{\{i,j\}}^s)} = \frac{p_{\{i,j\}}^s \left( y = \operatorname{argmax} \left[ \mathbf{z}'_{\{i,j\}} \right] \right)}{p_{\{i,j\}}^s \left( y = \operatorname{argmax} \left[ \mathbf{z}_{\{i,j\}}^s \right] \right)},$$

which is precisely the conditional posterior, and thus the acceptance probability reduces to  $A_{alloc}^{\{i,j\}} = 1, \forall \{i, j\} : i > k \in \mathcal{I}$ .
